# Supplementary material for: Learning Robust Dynamics through Variational Sparse Gating
Source: arXiv:2210.11698 source file (2022-10-21)
Supplement: Supplementary file 1 [file RelatedWork.tex]

\section{Extended Related Work}
\label{app:related_work}
\textbf{Latent Dynamics Models}: Latent dynamics models~\cite{bourlard2012connectionist, kalman1960filter, bengio1999markovian} operate directly on sequences predicted in the latent space rather than autoregressively feeding back the generated frames back to the model. Recent advancements in deep learning have allowed learning expressive latent dynamics models using stochastic backpropagation~\cite{kingma2013vae,chung2015vrnn, krishnan2015deepkalman, karl2016dvbf}. PLaNet introduced Recurrent State Space Models (RSSM)~\cite{hafner2018planet} where the latent dynamics models comprised of stochastic and deterministic components. VideoFlow~\cite{kumar2019videoflow} predicted future values of the latent state by normalizing flows for robotic object interactions.  Hierarchial latent models for video prediction were proposed in CWVAEs~\citep{saxena2021clockwork} with levels ticking at different intervals in time. \citep{franceschi2020stochastic,dona2021pdedriven} disentangled between dynamic and static factors. However, to get the static content like shape/color of objects, both of these methods used around 2-5 observations from the sequence. In partially observable setting, all the objects might not be visible in the sampled frames making it hard to estimate the static component. 

\textbf{Model-Based \gls{rl}}: Model-based RL methods train agents in a two-stage process. Firstly, a dynamics model of the environment is learned followed by learning of policy using imagined trajectories. SimPLe~\cite{kaiser2019simple} trains a PPO~\cite{schulman2017ppo} agent on the learned video generation model in pixel space. \Glspl{rssm} were proposed in PlaNet~\cite{hafner2018planet} where online planning was conducted in the latent space. SOLAR~\cite{zhang2018solar} solved robotics tasks via guided policy search in latent space. DreamerV1~\cite{hafner2019dreamer} learned behaviours by propagating analytic gradients of learned state values and achieved state-of-the-performance on DMControl Suite~\citep{tassa2018dmcontrol}. DreamerV2~\cite{hafner2020mastering} used categorical latents for the stochastic path and balanced the cross-entropy terms in the KL loss thereby achieving human-level performance on the Atari benchmark~\citep{bellemare2013ale}.

\textbf{Model-Free \gls{rl}}: Model-Free \gls{rl} learn policies directly from the observations received from the environment. Deep Deterministic Policy Gradient (DDPG)~\cite{lillicrap2015ddpg} combined actor-critic with insights from DQNs~\cite{mnih2015dqn} to learn agents for continuous action spaces. TD3~\cite{fujimoto2018td3} builds upon the DDPG algorithm and addresses the problem of overestimation bias in the value function. CURL~\cite{srinivas2020curl} uses contrastive losses to learn discriminative representations. DrQ~\cite{kostrikov2020drq} and  DrQ-v2~\citep{yarats2021drqv2} employed data augmentation techniques and do not use auxiliary losses or pre-training. 

\textbf{Sparsity in \gls{rnn}}:

\textbf{Environments}:
